# Supplementary material for: Deep ReLU Programming
Source: arXiv:2011.14895 source file (2021-03-08)
Supplement: Supplementary file 1 [file appendix.tex]

\section{Implementation}
\subsection{Helper functions}
\begin{lstlisting}
using Distributions

####################
# Function to generate random network 
# parameters for a given architecture
####################
function randomParameters(n0,n,L)
W=Array{Matrix{Float64},1}(L+1)
b=Array{Array{Float64,1},1}(L+1)
W[1]=rand(Uniform(-1,1),n[1],n0)
b[1]=rand(Uniform(-1,1),n[1])
for i = 2:L
	W[i]= rand(Uniform(-1,1),n[i],n[i-1])
	b[i]=rand(Uniform(-1,1),n[i])
end
W[L+1]=rand(Uniform(-1,1),1,n[L])
b[L+1]=rand(Uniform(-1,1),1)
return (W,b)
end


####################
# Define the neural network itself 
# and similar functions
####################
htilde(layerNum,input)= W[layerNum]*input+b[layerNum]
ReLU(x)=max(0,x)
h(l,x)=ReLU.(htilde(l,x))
function f(x)
	tmp=x
	for l = 1:L
		tmp=h(l,tmp)
	end
	return htilde(L+1,tmp)
end

####################
# function to compute the signature 
# at a given point x
####################
function signature(x)
	s=Array{Array{Bool,1},1}(L)
	tmp=x
	for l = 1:L
		tmp=htilde(l,tmp)
		s[l]=(tmp.>0)
		tmp=ReLU.(tmp)
	end
	return s
end

####################
# function to compute the signature 
# and the gradient at a given point x
####################
function sigGrad(x)
	s=Array{Array{Bool,1},1}(L)
	grad=eye(2)
	tmp=x
	for l = 1:L
		tmp=htilde(l,tmp)
		s[l]=(tmp.>0)
		grad=s[l].*W[l]*grad
		tmp=ReLU.(tmp)
	end
	grad=W[L+1]*grad
	return (s,grad[1,:])
end

####################
# the advancemax algorithm step at position x
# in direction v with signature s ignoring 
# signature changes in neurons specified in "critical"
####################
function advanceMaxAdjusted(x,v,s,critical=Array{Tuple{Int32,Int32,Array{Float64,1}},1}())
	sort!(critical,lt=sortfunction)
	criticalIdx=1;
	considerCritical=(criticalIdx<=length(critical))
	nextCriticalLayer=0;
	if considerCritical
		nextCriticalLayer=first(critical[criticalIdx])	
	end
	change=Array{Tuple{Int,Int,Bool},1}()
	sizehint!(change,10)
	α=W[1]*x+b[1]
	β=W[1]*v
	t=Inf64
	for i = 1:L
		for j = 1:n[i]
			if considerCritical
				if nextCriticalLayer==i
					if critical[criticalIdx][2]==j
						criticalIdx+=1
						if criticalIdx>length(critical)
							considerCritical=false
						else
							nextCriticalLayer=first(critical[criticalIdx])	
						end
						continue;
					end
				end
			end
			if β[j]!=0
				τ=-α[j]/β[j]
				if ((s[i][j]==true)&&(β[j]<0))||((s[i][j]==false)&&(β[j]>0))
					if τ<=t
						if τ<t
							empty!(change)
							t=τ
						end
						push!(change,(i,j,(β[j]>0)))
					end
				end
			end
		end
		α= W[i+1]*(s[i].*α)+b[i+1]
		β= W[i+1]*(s[i].*β)
	end
	return (t,change)
end

####################
# compute the gradient at "x" with signature 
# changed as specified in "change"
####################
function adjustedSGrad(x,change=Array{Tuple{Int64,Int64,Bool},1}())
	s=Array{Array{Bool,1},1}(L)
	sort!(change,by=first)
	changeIdx=1;
	considerChanges=(changeIdx<=length(change))
	nextChangeLayer=0;
	if considerChanges
		nextChangeLayer=first(change[changeIdx])	
	end
	α=W[1]*x+b[1]
	γ=W[1] 
	for i = 1:L
		sLayer=(α.>0)
		if considerChanges
			while nextChangeLayer==i 
				sLayer[change[changeIdx][2]]=change[changeIdx][3]
				changeIdx+=1
				if changeIdx>length(change)
					considerChanges=false
					break;	
				end
				nextChangeLayer=first(change[changeIdx])	
			end
		end
		α= W[i+1]*(sLayer.*α)+b[i+1]
		γ= W[i+1]*(sLayer.*γ)
		s[i]=sLayer
	end
	return (s,γ[1,:])
end

function sortfunction(x,y)
	if x[1]<y[1]
		return true;
	elseif x[1]==y[1]
		if x[2]<y[2]
			return true;
		end
	end
	return false
end

####################
# determine critical vectors at "x" with specified signature "s", 
# i.e. directions in which the signature would change immediately
####################
function determineCritical(x,s,epsilon=1e-10)
criticalVectors=Array{Tuple{Int32,Int32,Array{Float64,1}},1}()
α=W[1]*x+b[1]
γ=W[1] 
for i = 1:L
for j = 1:n[i]
	σ=dot(γ[j,:],γ[j,:])
	if σ>0&&(abs(α[j]/σ)<epsilon)
		push!(criticalVectors,(i,j,γ[j,:]))
	end
end
α= W[i+1]*(s[i].*α)+b[i+1]
γ= W[i+1]*(s[i].*γ)
end
return (criticalVectors)
end

function subtractOrthogonal(subtractFrom,crit,s)
res=subtractFrom;
orthogonal=Array{Array{Float64,1},1}()
used = fill(false,length(crit))
sizehint!(orthogonal,length(crit))
finished=false;
while finished==false 
	finished=true;
	for i = 1:length(crit)
		u=crit[i][3]
		l=crit[i][1]
		j=crit[i][2]
		if !used[i]&&(((s[l][j]==true)&&(dot(u,res)<0))||
					  ((s[l][j]==false)&&(dot(u,res)>0)))
			for j = 1:length(orthogonal)
				w=orthogonal[j]
				u=u-dot(u,w)*w
			end
			if abs(dot(u,u))>epsilon
				finished=false
				u=(1/sqrt(dot(u,u)))*u
				push!(orthogonal,u)
				res=res-dot(res,u)*u
			end
		end
	end
end
return res
end
\end{lstlisting}
\subsection{Sample usage}
\begin{lstlisting}
using Plots
Plots.pyplot()


include("algorithm.jl")


####################
# Define the network and similar functions
####################
n0=2
L=8
n=rand(10:50,L)
(W,b)=randomParameters(n0,n,L)
#
epsilon=1e-10
x=rand(Uniform(-5,5),2);
#= x=[1.0,0.5] =#
crit= Array{Tuple{Int32,Int32,Array{Float64,1}},1}()
(s,grad)=sigGrad(x);
v=-grad
(t,change)=advanceMaxAdjusted(x,v,s,crit)
x=x+t*v
(s,grad)=sigGrad(x);
count=0;
while true
	println("___")
	println("change=$change")
	println("x=$x  f(x)=$(f(x))")
	#######
	# compute adjusted signature and gradient at x based on signature changes
	#######
	(s,adjustedgrad)=adjustedSGrad(x,change);
	v2=-adjustedgrad
	println("adjustedgrad=$adjustedgrad")
	crit=determineCritical(x,s)
	#######
	# orthogonalize
	#######
	println("Number orthogonalizing vectors:$(length(crit))")
	v = subtractOrthogonal(v2,crit,s)
	#= println("gradNormalized=$gradNormalized") =#
	#= v=-gradNormalized =#
	if dot(v,v)<epsilon
		if count<10
			empty!(change)
			for t = crit
				if(rand([0,1],1)[1]==1)
					#= println("AAA $t") =#
					push!(change,(t[1],t[2],!s[t[1]][t[2]]))
				end
			end
			#= println("AAA change=$change") =#
			count+=1
			continue;
		else
			break
		end
	else
	(t,change)=advanceMaxAdjusted(x,v,s,crit)
	f(x)
	f(x+t*v)
	x=x+t*v
	count=0;
	#= sleep(0.1) =#
	end
end


closeall()

#= plotfun2(x)=dot(adjustedgrad,x) =#
plotfun=f
#= plotfun=plotfun2 =#
x
env=0.25
xrange=[x[1]-env,x[1]+env]
yrange=[x[2]-env,x[2]+env]
#= plotF(xrange,yrange) =#
#= function plotF(xrange,yrange) =#
res = 50
xvals = linspace(xrange[1],xrange[2], res)
yvals = linspace(yrange[1],yrange[2], res)
#= y = x =#
z = Array{Float64}(res, res);
for i in 1:res
    for j in 1:res
		z[j, i] = (plotfun([xvals[i], yvals[j]]))[1];
    end
end
Plots.surface(xvals, yvals, z')
#= end =#
\end{lstlisting}
